# Supplementary material for: Masked Adversarial Generation for Neural Machine Translation
Source: arXiv:2109.00417 source file (2021-09-01)
Supplement: Supplementary file 1 [file appendix.tex]

\section{Gradient Analysis} \label{sec:gradient_analysis}
We decided to analyse the relation between different type of attacks and the true increase in loss on the WMT14 de-en validation split. This split is roughly 7000 sentences.
%We also did the same experiment on the train and test splits. Since the figures are very similar, we will only present the validation split's results.
First, we compare the approximation of change in loss to the real change in loss with a white box adversarial substitution on a trained transformer model.
Then we compare the real change in loss with the following attacks. All of which correspond to the substitution of a single word in the sentence, either on the source side or the target side.
\begin{itemize}
    \item \textbf{adv} :  Both the position and the substitute word are chosen adversarially as in \ref{pert}.
    \item \textbf{random pos} : The position is chosen randomly and the substitute word adversarially.
    % \item \textbf{random voc} : The position is chosen adversarially as in \ref{pert} and the substitute word is chosen randomly.
    \item \textbf{gnorm pos} : The position $\tilde{i}$ is chosen such as $\tilde{i}=\mathrm{arg}\max_i \Vert \nabla_{e_i}\mathcal{L}\Vert_2$. The substitute word is chosen at random.
    \item \textbf{random} : Both the position and the substitute word are chosen at random.
\end{itemize}
Finally we compare $\epsilon = \Vert \tilde{e_i} - e_i \Vert$ across these attacks. This corresponds to the force of the attack in the embedding space.

\begin{figure}[hbt!]
    \centering
    \includegraphics[width=7cm]{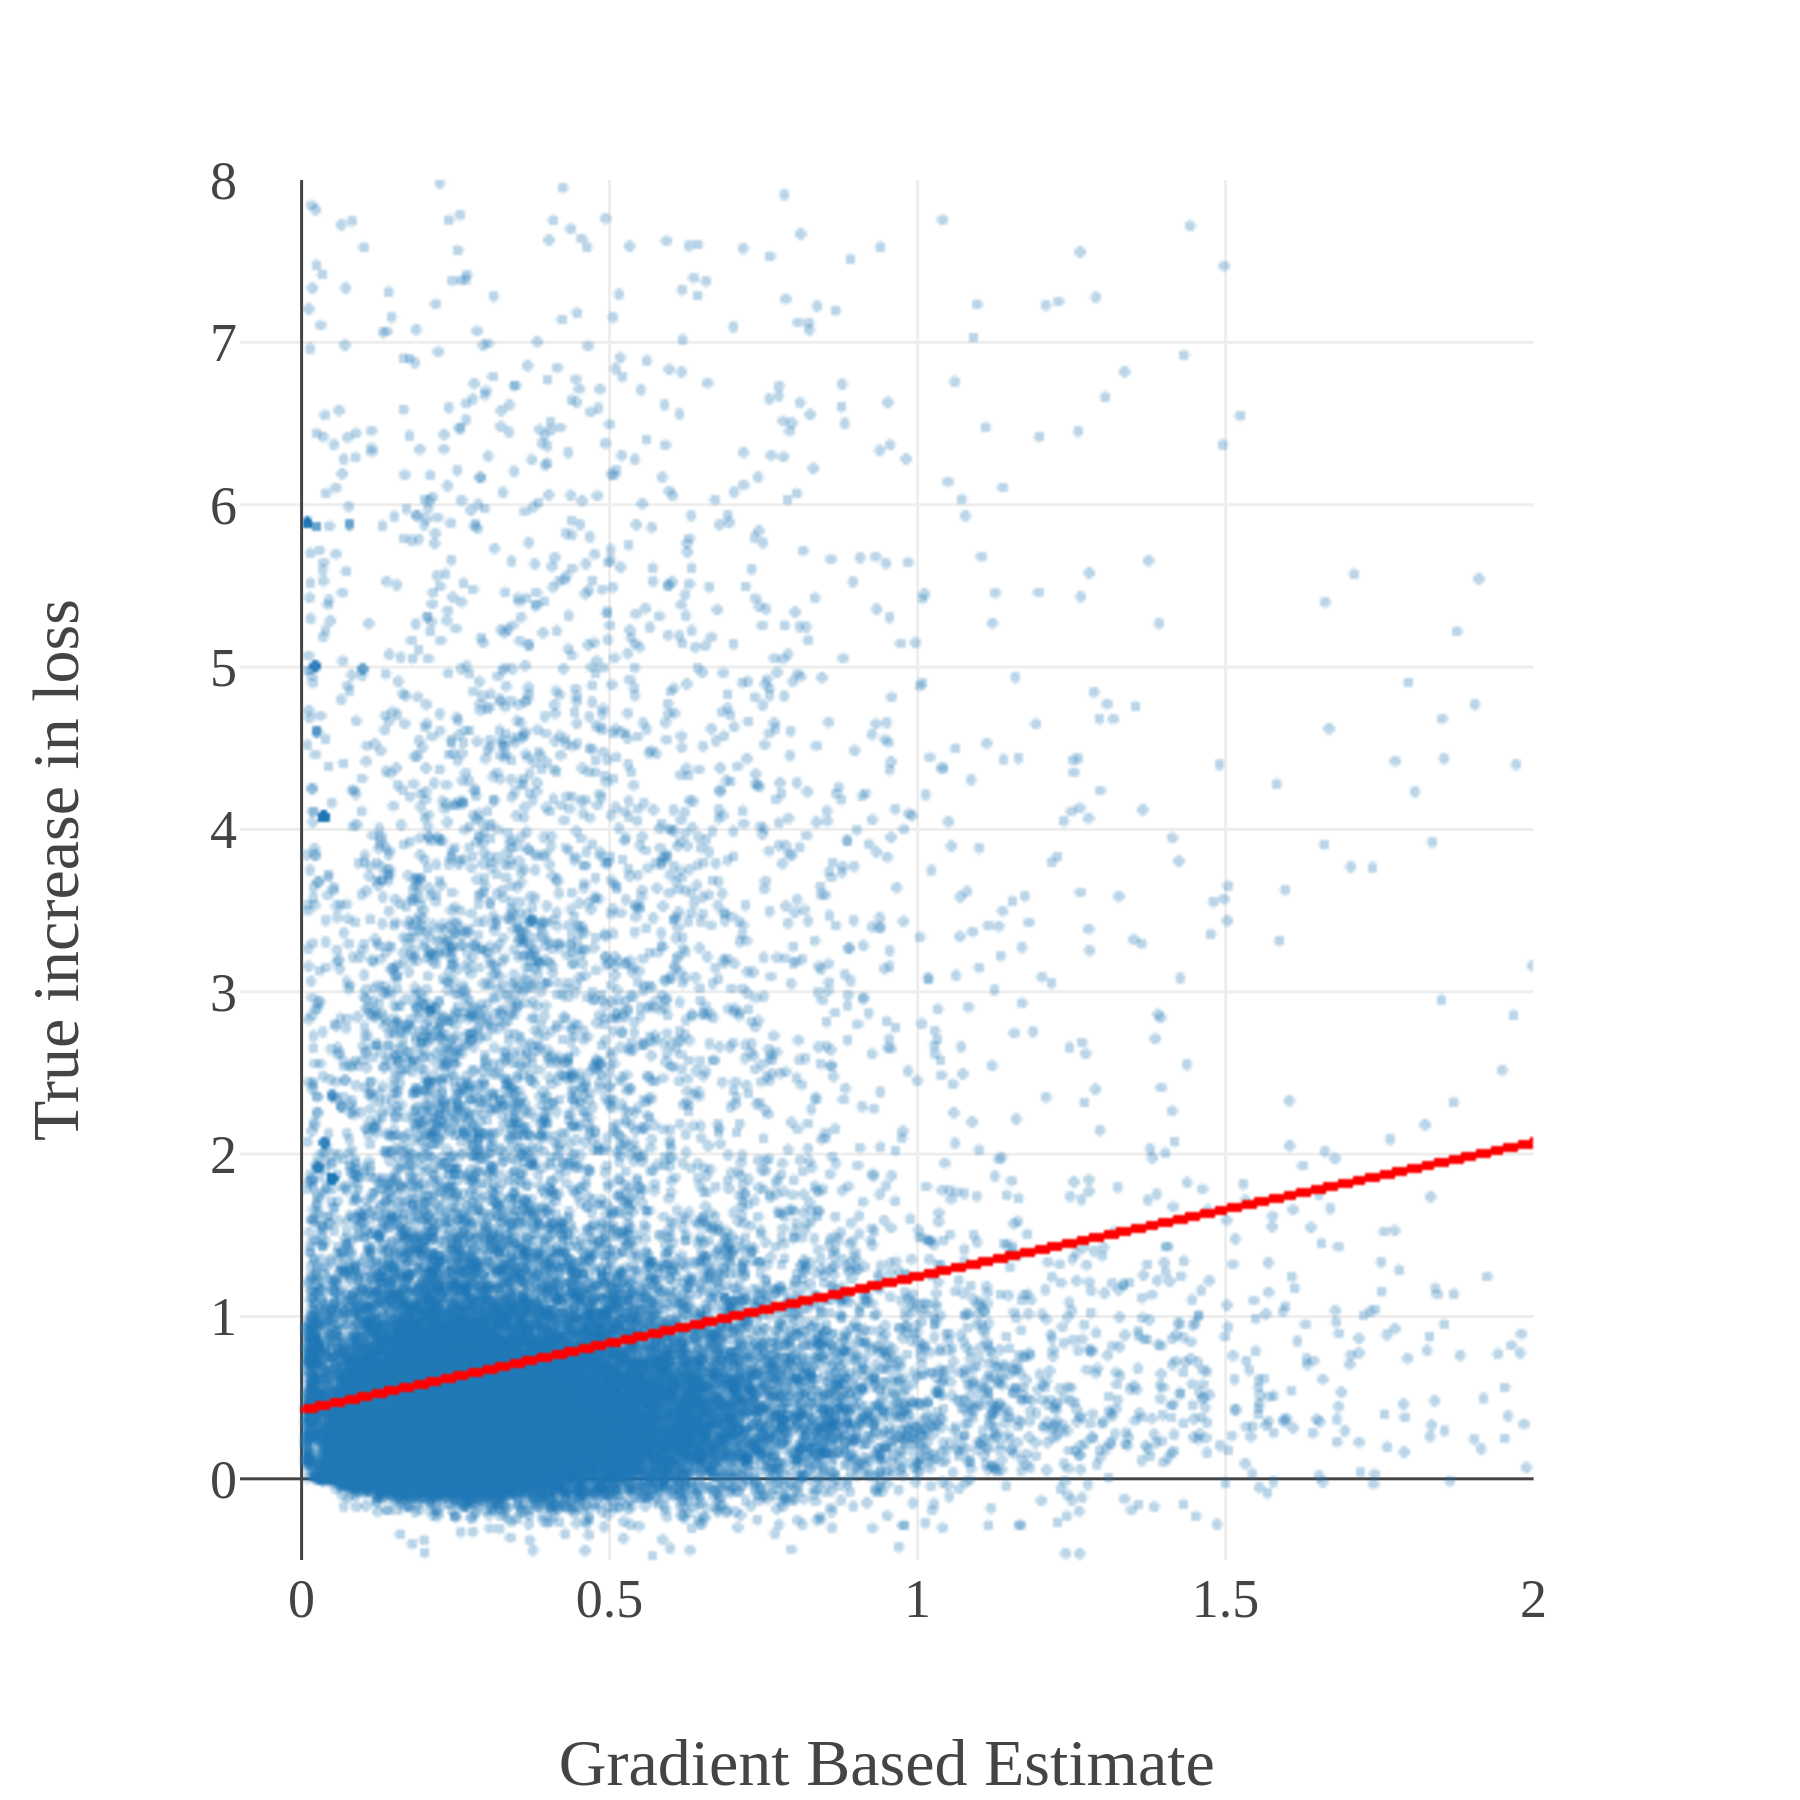}
    \caption{Comparing the distribution of the true increase in loss and its gradient-based estimate and their correlation, using
    best flips for each \textbf{source} sentence on WMT14 validation dataset. Linear regression gives $\text{True increase in loss} = 0.82\times\text{Gradient based estimate} + 0.42$ with $R^2=0.03$}
    \label{fig:approx}
\end{figure}
%\todo{Is this plot impacted by the vocab issue ?}

Figure \ref{fig:approx} shows that the approximation in equation \ref{approx} is far from being verified. Indeed there is only a Pearson correlation of $0.176$ between the two variables.
However, the gradient could still be useful if it consistently leads us to neighboring regions of higher loss better than a \textbf{random} attack.

\begin{figure*}
    \centering
    \includegraphics[width=0.9\textwidth]{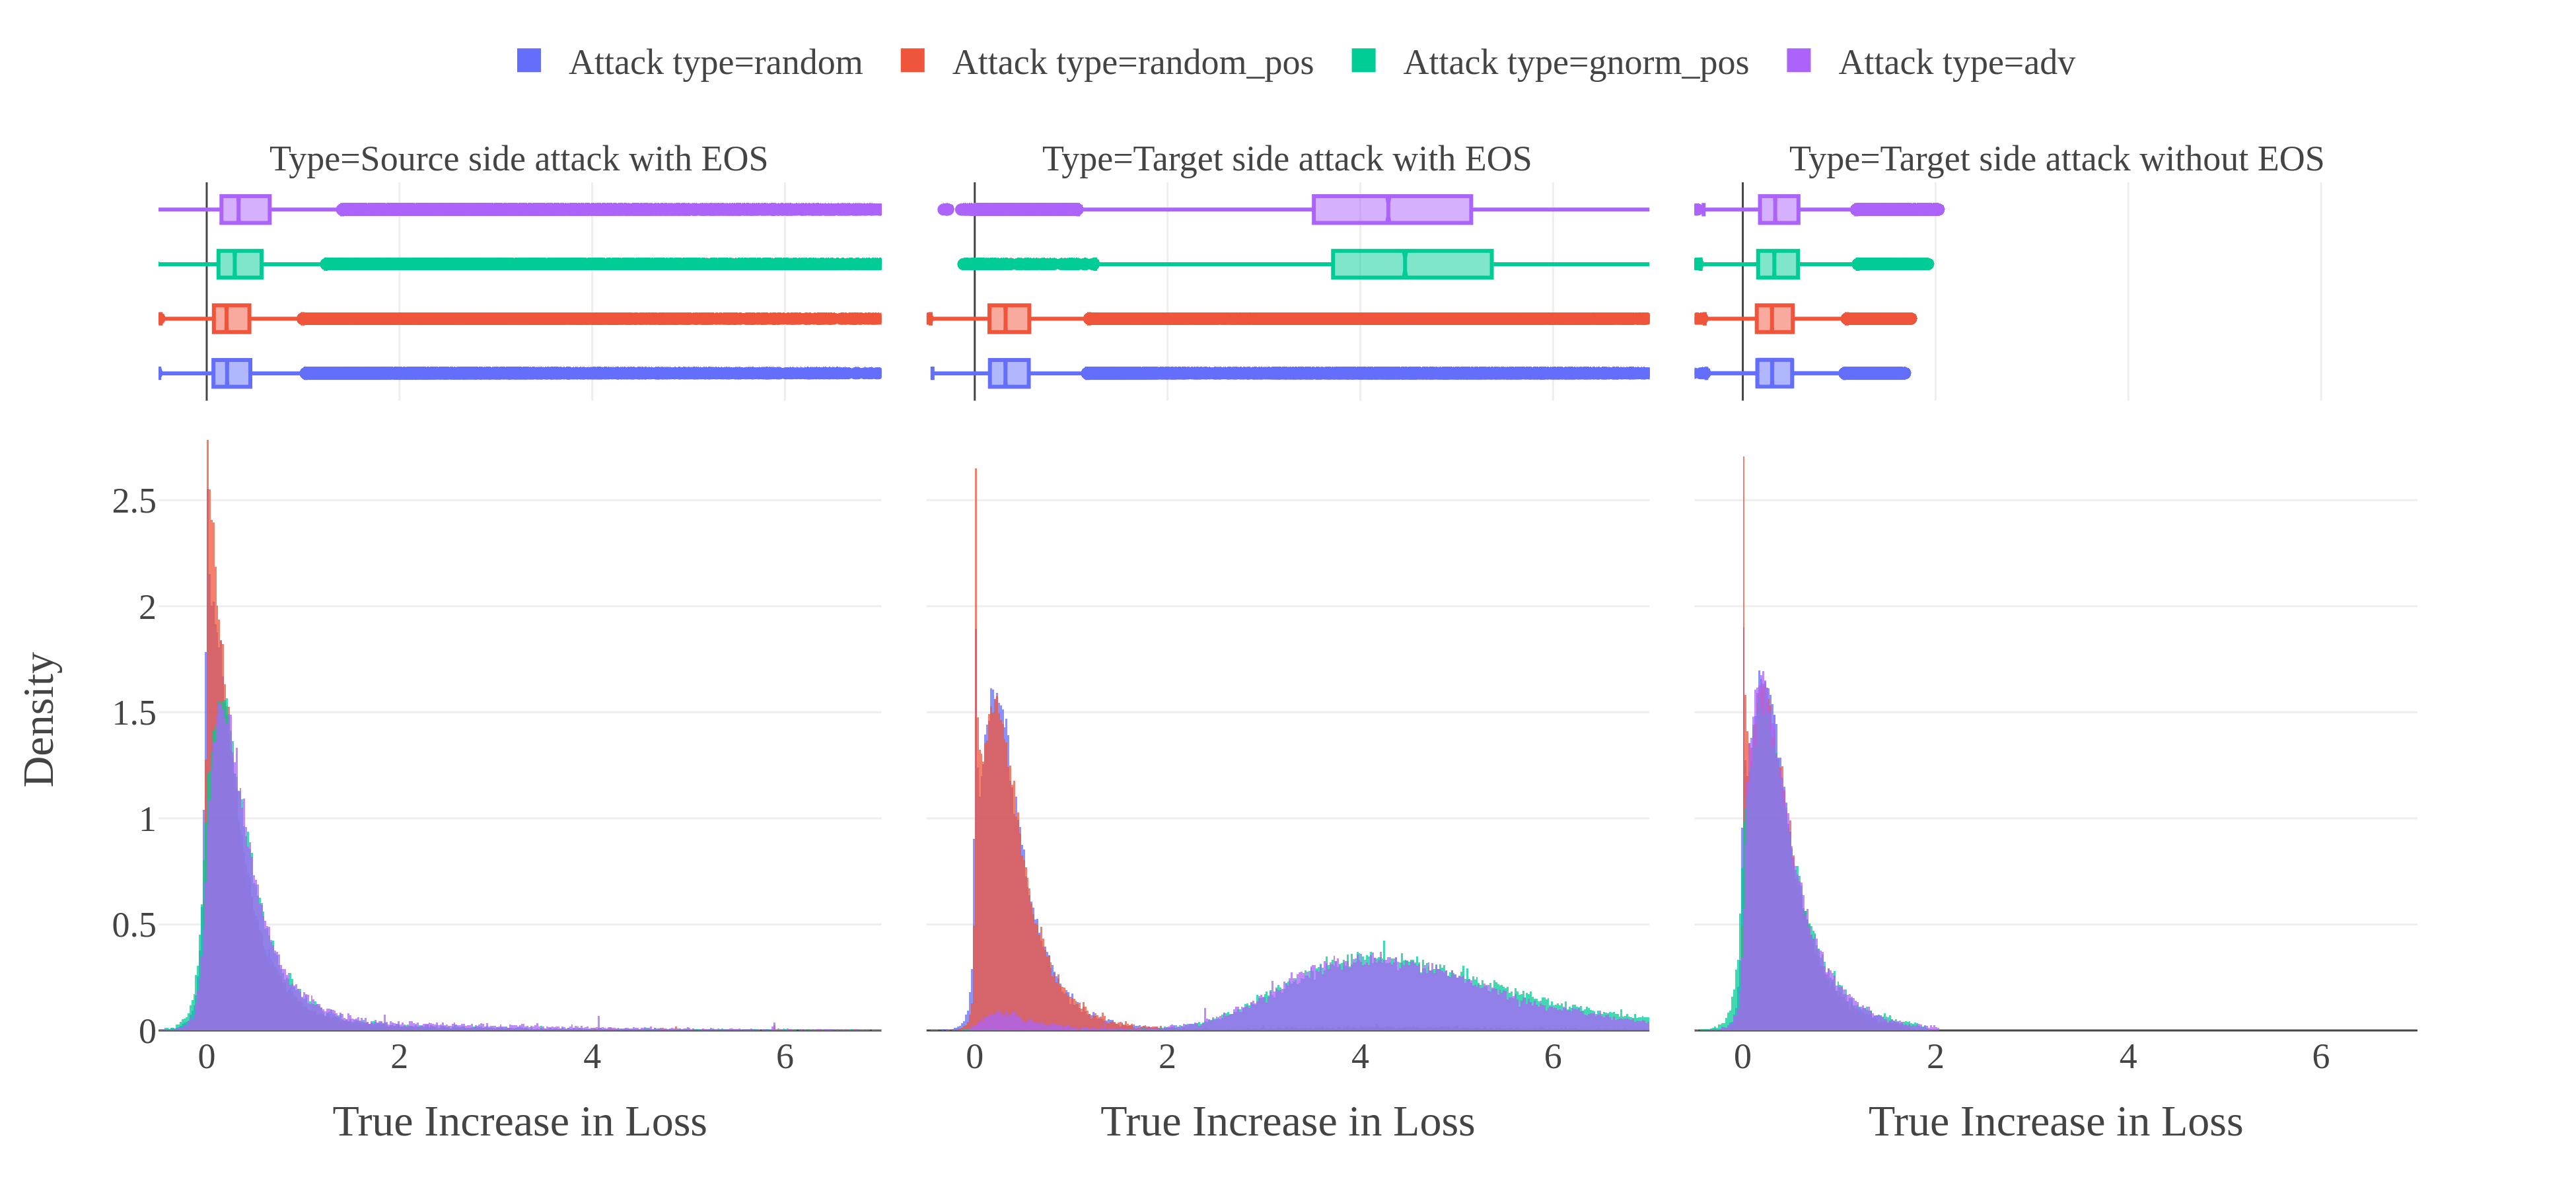}
    \caption{Comparing the impact on loss of different attacks on the source side and target side. The two left plots allow the attacks to change the EOS special token. The last plot protects the EOS (End of Sentence) token from being changed.}
    \label{fig:comparison_random}
\end{figure*}  

Figure \ref{fig:comparison_random} shows us that on the source side, the whitebox adversarial attacks \textbf{adv}, \textbf{random pos} and \textbf{gnorm pos} have a very similar effect on the loss compared to the fully \textbf{random} method.
On the target side however, there is a significant increase in attack efficiency when comparing \textbf{adv} and \textbf{gnorm pos} to \textbf{random} and \textbf{random pos}. 
It turns out that this is due to the sensitivity of the model to changes on the special token EOS. 
As shown in the right subplot in figure \ref{fig:comparison_random}, protecting the EOS token nearly removes all the difference between the adversarial methods and the random attack.
In our experiments, training a model on a random perturbation also had the effect of removing the sensitivity to EOS, giving very similar results to protecting the EOS token.
In all our experiments, \textbf{random pos} and \textbf{random} were almost equivalent, with a pearson correlation of 0.9. 
\textbf{gnorm pos} which only uses the position information to attack is also very close to the fully adversarial attack \textbf{adv}.
This lets us conclude that the word with which we substitute has little effect on the attack strength. The position to perturb is the most important. However, adding a random word
may add too much noise in the translation model.
%However in all cases except when perturbing EOS, the white box adversarial attacks aren't very efficient and the additional overhead in training doesn't justify the very small improvement in attack efficiency. 
%Training methods like doubly adversarial inputs and AdvAug give significant improvements because of the rich data augmentation generated by the language models and mixup in the case of AdvAug.

\begin{figure}
    \centering
    \includegraphics[width=0.5\textwidth]{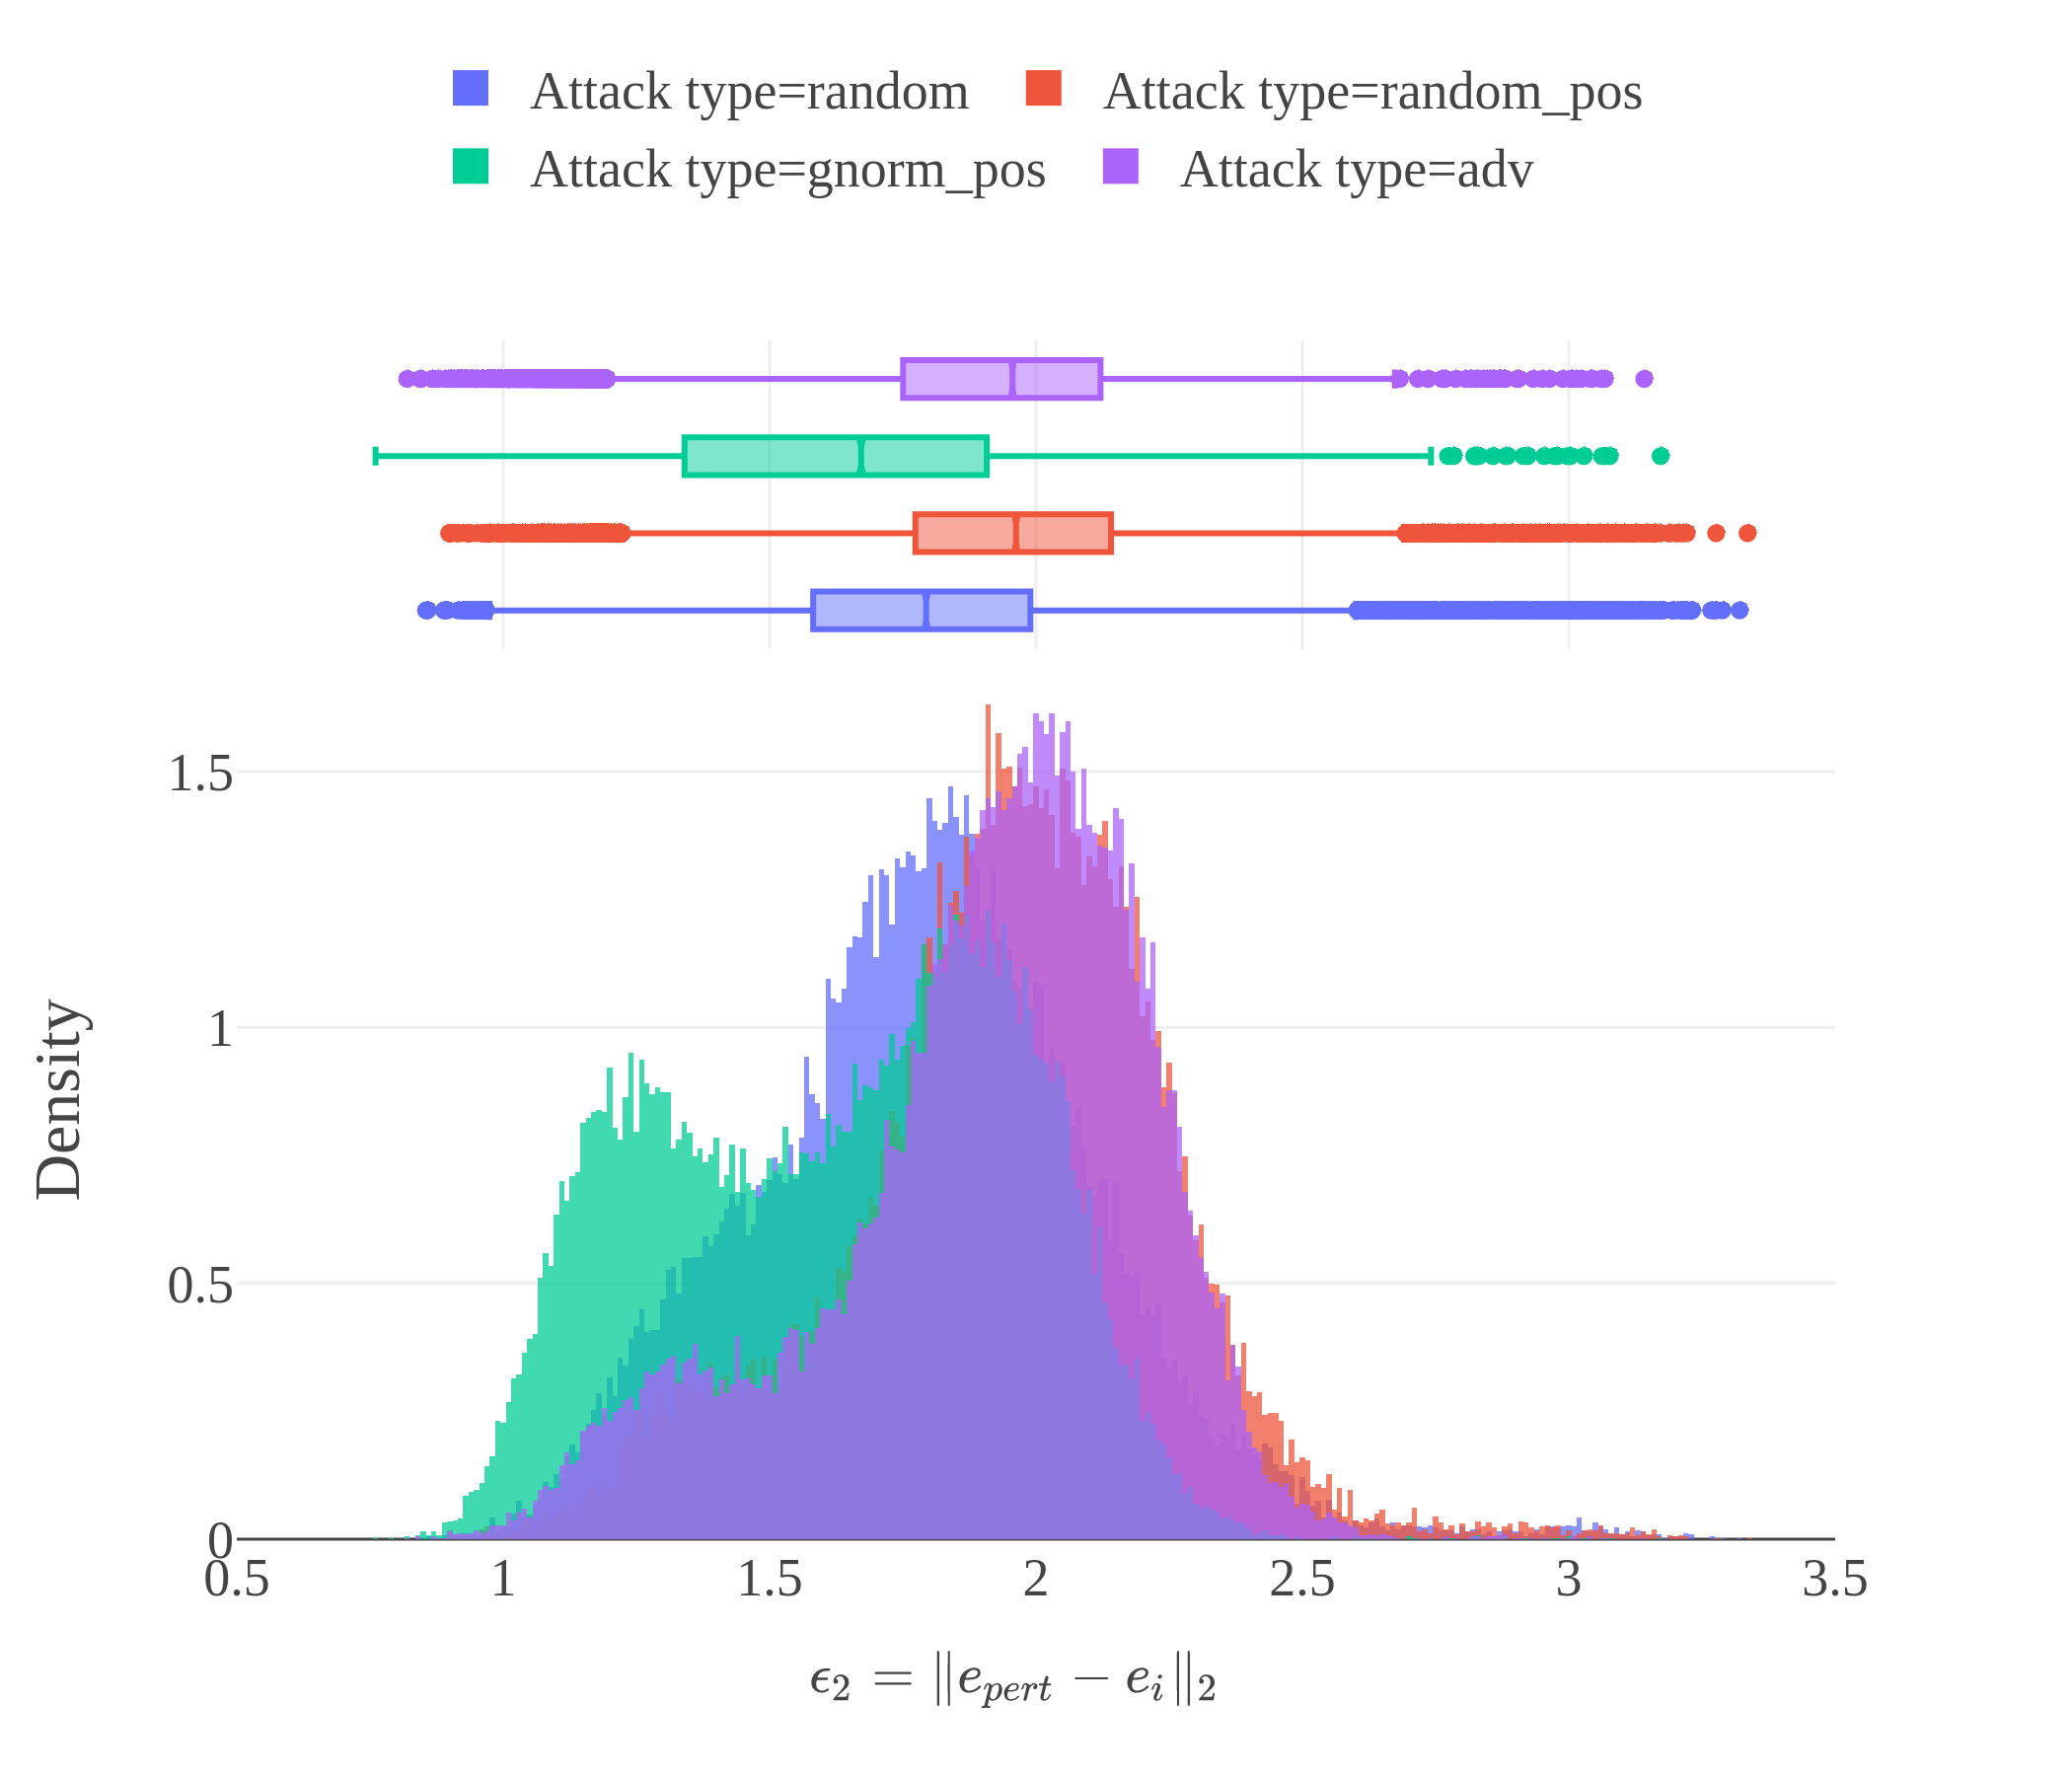}
    \caption{Distribution of the size of perturbation given an attack. The $\mathbb{L}_2$ norm of a word embedding vector is usually around 2}
    \label{fig:epsilon}
\end{figure}

\subsection{Adversarial Attack and Defense in Computer Vision}
For the readers interested in robustness in computer vision, we include here short review of the field.
Robustness is a rapidly growing field of research in machine learning. 
Neural Networks have impressive performances on several benchmarks, even surpassing human baselines. 
However, they still behave very strangely on some inputs. 
Famously, Szegedy et al \cite{szegedy2014} showed that by maximizing the classification error of a neural network, we can find imperceptible perturbations that completely change the output of the model. 
These inputs are now known as \textit{adversarial} examples. 
The existence of these inputs and many others, show that neural networks are very brittle and sensitive to slight changes in the input. 

The study of these adversarial examples gave rise to the new field of adversarial attack. Many attacks have been proposed. Some of the notable adversarial attacks in the context of this work are : 
\begin{itemize}
    \item The Fast Gradient Sign Method takes a gradient ascent step on the input and then clamps the perturbation to the $\epsilon \ell_{\infty}$ ball \cite{goodfellow2015}. The advantage of this attack is its computational efficiency.
    \begin{equation*}
        \boldsymbol{\eta}=\epsilon \operatorname{sign}\left(\nabla_{\boldsymbol{x}} L(\boldsymbol{\theta}, \boldsymbol{x}, y)\right)
    \end{equation*}
    
    \item Projected Gradient Descent (PGD) \cite{madry2017} takes multiple gradient descent steps to maximize the loss and projects back to the $\epsilon$ ball at each step. Naturally, the more steps are taken, the more successful the attack is.
    \begin{equation*}
    x^{t+1}=\Pi_{x+S}\left(x^{t}+\epsilon \operatorname{sign}\left(\nabla_{x} L(\theta, x, y)\right)\right)
    \end{equation*}
\end{itemize}

The existence of these adversarial examples isn't very surprising when we consider that the optimization is only performed on the expected value. 
The model doesn't need to be robust to these inputs to perform well.
Expected Risk Minimization does the following optimization : 

\begin{equation*}
    \min_{\theta}\mathbf{E}_{(x, y) \sim \mathcal{D}_{\text{train}}} L(\theta, x, y)
\end{equation*}

With $x$ a continuous input, $y$ a label, $\theta$ the parameters and $L$ the loss function. 
To counteract the adversarial attacks, robust optimization was introduced. 
Contrary to the usual Expected Risk Minimization, robust optimization trains the model in the worst-case scenario : 

\begin{equation*}
    \min_{\theta}\mathbf{E}_{(x, y) \sim \mathcal{D}}\left[\max _{\delta \in \Delta(x)} L(\theta, x+\delta, y)\right]
\end{equation*}

This min-max problem is solved in practice by first finding $\delta^*$ that maximizes the loss at $x$ and then applying the usual gradient descent on the loss $L(\theta, x + \delta^*, y)$. 
This last property is given by Danskin’s theorem in optimization. \cite{madry2017}

In their paper, Madry et al \cite{madry2017} propose to train a robust classifier by generating adversarial examples using the PGD algorithm. They succeed in training a classifier that resists to attacks that are even stronger than the ones the classifier was trained on. 

The research on the subject is a back and forth between developing strong attacks that break current defenses and developing defenses that are hard to break. These studies are similar to what can be seen in cybersecurity research, where a threat model should be clearly defined. The characteristics of the attack need to be clear : its goal, knowledge available to it and its capabilities. 
For example, a Computer Vision attack's goal could be to alter the model's prediction $y\ne y_{target}$.
The attack could be white box : it has access to the model weights.
Finally it could alter the input very slightly ($\mathcal{L}_\infty$ for example). \cite{carlini2019}

A set of best practices for research in this subject was compiled by prominent researchers in the field \cite{carlini2019} and one important point was to develop defenses that we actively try to break. As Feynman concisely put it, “the first principle [of research] is that you must not fool yourself—and you are the easiest person to fool.”

One notable example of this is gradient masking \cite{tramer2018}. 
Single-step adversarial training (with FGSM) leads to distorting the loss landscape locally. 
It makes the gradients very small on the training points. 
It therefore prevents the single-step gradient attacks from generating adversarial examples. 
However it fails to make the model more robust against stronger adversaries that escape the local minimum.   

When these adversarial examples were discovered in \cite{szegedy2014}, it was hypothesized that these examples stemmed from the high non-linearity of neural networks. However, \cite{goodfellow2015} shows that it is in fact the high dimensionality of the linear transformations that might be the root of the problem. 
Indeed, small perturbations on the input tend to cancel out statistically with the transformation when they are random, but carefully crafted perturbations can add up and result in a big change in output. 

Robust training with PGD was for a while the most robust way of training neural networks, but the multiple steps required made training orders of magnitude slower. 
This makes it very hard to use PGD training in very large networks such as those used in Neural Machine Translation. A few other methods made this process faster :
\begin{itemize}
    \item You Only Propagate Once (YOPO) \cite{zhang2019} uses Pontryagin's Maximal Principle to restrict the forward and backward passes to the first layer, greatly reducing the computational cost. 
    \item Free Adversarial Training \cite{shafahi2019} takes advantage of the multiple PGD steps to accumulate the network's parameter gradients and thus converges much faster.
    \item Fast is Better than Free \cite{wong2019} surprisingly shows that FGSM training with random initial perturbations performs just as well as PGD and can resist to stronger multi-step PGD attacks. 
\end{itemize}

Virtual Adversarial Training \cite{miyato2019} approaches the problem a little differently. Miyato et al attack the model by trying to change the output probability distribution as much as possible. They do this by generating an input that maximizes the Kullback-Leibler divergence between the perturbed and unperturbed output distributions. This has the effect of smoothing the output distribution around a given point. It also has the benefit of not requiring labels and thus can be applied in a semi-supervised context. 

In computer vision, there is a certain trade-off between robustness and accuracy that has been proven empirically by Tsipras et al \cite{tsipras2018} and later theorized by Zhang et al \cite{zhang2019b}. Training a robust classifier leads to a drop in accuracy. However, Tsipras et al also showed that this drop in accuracy also comes with the added benefit of learned features that align better with human perception.
